# Supplementary material for: UniLayDiff: A Unified Diffusion Transformer for Content-Aware Layout Generation
Source: arXiv:2512.08897 source file (2026-09-11)
Supplement: Supplementary file 1 [file abl_losses.tex]

\begin{table}[t]
% \vspace{-6pt}
\centering
\setlength{\tabcolsep}{4pt}

 % 调整行距
\resizebox{\linewidth}{!}{
\begin{tabular}{lcccccc}
\toprule
$\lambda_{\mathrm{1}}$  & Occ~$\downarrow$ & Rea~$\downarrow$  & Und\mysub{S}~$\uparrow$ & Ove~$\downarrow$& FID~$\downarrow$ &Vio\%$\downarrow$\\
\midrule

0.05    &   0.115   &   0.0127   &   0.884   &   0.0040   &  2.24 & 29.6  \\

0.1    &   0.123   &   0.0129   &   0.885   &   0.0042   &  2.41  & 25.2 \\

\rowcolor{lightblue}0.2(Ours) &  0.119    &   0.0131   &  0.883    &   0.0049   &   2.15  & 22.4\\

0.5  &  0.122    &   0.0135   &  0.876   &  0.0056   &    2.96 &  21.3\\

\bottomrule
\end{tabular}
}
\vspace{-5pt}
\caption{Ablation study on different coefficient values for $\mathcal{L}_{\mathrm{rel}}$ term on the PKU annotated dataset, evaluated using the relationship task.}
\label{tab:lrel}
\vspace{-8pt}
\end{table}

\begin{table}[t]
% \vspace{-6pt}
\centering
\setlength{\tabcolsep}{8pt}
 % 调整行距
\resizebox{\linewidth}{!}{
\begin{tabular}{lccccc}
\toprule
$\lambda_{\mathrm{2}}$  & Occ~$\downarrow$ & Rea~$\downarrow$  & Und\mysub{S}~$\uparrow$ & Ove~$\downarrow$ &FID~$\downarrow$\\
\midrule

0.2    &   0.135   &   0.0129   &  0.964    &  0.0015    &   2.54   \\

\rowcolor{lightblue} 0.4\textbf{(Ours)} &   0.128   &   0.0129   &  0.963    &   0.0018   &   3.09   \\

1  &   0.125   &  0.0125    &    0.958  &   0.0023   &   3.42    \\

\bottomrule
\end{tabular}
}
\vspace{-5pt}
\caption{Ablation study on different coefficient values for $\mathcal{L}_{\mathrm{ctn}}$ term on the PKU annotated dataset, using the C $\rightarrow$ S + P task.}
\label{tab:lctn}
\vspace{-8pt}
\end{table}

\begin{table}[t]
% \vspace{-6pt}
\centering
\setlength{\tabcolsep}{8pt}
 % 调整行距
\resizebox{\linewidth}{!}{
\begin{tabular}{lccccc}
\toprule
$\lambda_{\mathrm{3}}$  & Occ~$\downarrow$ & Rea~$\downarrow$  & Und\mysub{S}~$\uparrow$ & Ove~$\downarrow$ &FID~$\downarrow$ \\
\midrule

0.2    &   0.114   &  0.0118    &   0.992   &  0.0006    &   3.36   \\

0.5    &   0.113   &   0.0119   &  0.994     & 0.0007    &   3.28   \\

\rowcolor{lightblue} 1\textbf{(Ours)} &   0.115   &   0.0114   &  0.996    &  0.0005    &  3.15    \\

2  &   0.116   &  0.0115    &  0.998    &   0.0009   &   3.44   \\

\bottomrule
\end{tabular}
}
\caption{Ablation study on different coefficient values for $\mathcal{L}_{\mathrm{und}}$ term. on the PKU annotated dataset, evaluated using the unconditional generation task.}
\label{tab:lund}
\vspace{-8pt}
\end{table}
