# Supplementary material for: UniLayDiff: A Unified Diffusion Transformer for Content-Aware Layout Generation
Source: arXiv:2512.08897 source file (2026-09-11)
Supplement: Supplementary file 2 [file adaln.tex]

\begin{table}[t]
\centering
\fontsize{10}{10}\selectfont
\setlength{\tabcolsep}{5pt}
\resizebox{\linewidth}{!}{
\begin{tabular}{cc cccccc}
\toprule
Salbox & Image & Occ$\downarrow$ & Rea$\downarrow$ & Und$_S\uparrow$ & Ove~$\downarrow$ & FID~$\downarrow$ \\
\midrule
\ding{55} & \ding{55} & 0.127 & 0.0131 & 0.994 & 0.0006 & 4.61 \\
\ding{51} & \ding{55} & 0.124 & 0.0126 & 0.983 & 0.0007 & 3.61  \\
\midrule
\rowcolor{lightblue}\ding{51} & \ding{51} & 0.122 & 0.0120 & 0.992 & 0.0005 & 3.37 \\
\bottomrule
\end{tabular}
}
\vspace{-0.3cm}
\caption{Ablation study on the impact of different visual guidance components (Saliency Box and Image) injected via adaLN-Zero on the PKU annotated dataset, evaluated using the unconditional generation task with pre-trained models.}
\vspace{-0.3cm}
\label{tab:adaln}
\end{table}
